# Supplementary material for: NSM4D: Neural Scene Model Based Online 4D Point Cloud Sequence Understanding
Source: arXiv:2310.08326 source file (2023-10-12)
Supplement: Supplementary file 1 [file supp.tex]

\appendix

In this document, we provide a list of supplementary materials to support the main paper.

\textbf{More experiment and ablation results.} In Section \ref{sec:exp}, we provide more experiment and ablation results to demonstrate our work's ability and superior property.

\textbf{Visualization.} In Section \ref{sec:vis}, we provide some visualization results of NSM4D to visualize the effects of our approach.

% \textbf{Detailed method.} We give a more comprehensive illustration of our method in Section \ref{sec:method}. We will provide detailed and concise notations. We believe this will help others to reproduce our work.

\textbf{Implementation details.} We additionally provide implementation details in Section \ref{sec:imp}.

% \textbf{Broader impacts.} We discuss the broader impacts of our work in Section \ref{sec:broader}.

\textbf{Limitations and future work.} In Section \ref{sec:lim}, we discuss the limitations of our work. We also list possible directions for future work to explore.

\section{More Experiment and ablation Results}
\label{sec:exp}
\subsection{Synthia 4D dataset}
In this section, we provide a complete comparison with previous work on Synthia 4D\citep{synthia} dataset. As shown in the table below,  when introducing our method, constant improvement is shown over vanilla PPTr in an online manner, demonstrating that our neural scene model is indeed customized for online 4D perception.
It further indicates that the compact and structured 4D history summary proposed in our paper is noticeably effective.
\begin{table}[h]
\setlength{\tabcolsep}{1.5mm}
\tiny{
\begin{center}
\begin{tabular}{l|c|cccccccccccc|c}
\hline\noalign{\smallskip}
Method & Frames & Bldn& Road& Sdwlk & Fence& Vegittn & Pole & Car & T.Sign & Pedstrn & Bicycl & Lane & T.Light& mIoU\\
\noalign{\smallskip}
\hline
\noalign{\smallskip}
% P4Transformer & 3(offline) & 96.73 & 98.35 & 94.03 & 95.23 & 98.28 & 98.01 & 95.60 & 81.54 & 85.18 & 0.00 & 75.95 & 79.07 & 83.16\\
PPTr & 3(offline) & \textbf{97.51} & 98.21 & \textbf{95.11} & \textbf{96.81} & \textbf{99.65} & 97.86 & \textbf{98.01} & 80.98 & \textbf{90.60} & 0.00 & 78.21 & 76.89 & 84.15 \\
% \noalign{\smallskip}
% \hline
\noalign{\smallskip}
% P4Transformer & 3(online) & 94.44 & 98.25 & 90.84 & 94.79 & 97.28 & 98.08 & 95.33 & 81.26 & 82.75 & 0.00 & 77.66 & 80.74 & 82.62 \\
PPTr & 3(online) & 94.68 & 98.32 & 93.11 & 95.26 & 97.30 & 98.06 & 95.42 & 82.74 & 85.55 & 0.00 & \textbf{78.31} & 81.70 & 83.37 \\
\noalign{\smallskip}
\hline
\noalign{\smallskip}
\tiny{+NSM4D} & 3(online) & 97.02 & \textbf{98.58} &94.01 & 95.82 & 97.80& \textbf{98.21} & 96.37 & \textbf{84.91} & 88.59& 0.00& 77.82 & \textbf{82.72} & \textbf{84.32} \\
\noalign{\smallskip}
\hline
\end{tabular}
\vspace{2mm}
\caption{Evaluation for online semantic segmentation on Synthia 4D dataset}
\vspace{-6mm}
\end{center}
}
\label{table:synthiamore}
\end{table}

\subsection{Robust to Noise.}
Our neural scene model is updated with the guidance of scene flow estimated from point clouds. To enhance the robustness of our module to noise induced during the flow estimation process, we adopt the average flow of the points within a token when updating. This approach reduces the performance degradation caused by noise accumulation in the sequences. We conducted experiments to verify the robustness of our method, as flow estimation is a crucial aspect of our framework. Results show that our method is highly robust to noise induced from the estimated flow. Specifically, while using ground truth scene flow yields a performance 68.66, our method only has a 0.88\% lower performance with the estimated flow.

\subsection{Number of tokens.}
The number of tokens controls the granularity of dynamic modeling. Not enough tokens might only focus on some local regions, lacking the ability to represent the whole scene. Increasing the number of tokens can maintain more fine-grained details in the scene model, but it leads to more memory overhead and less robustness to random noise. We compare different numbers of tokens in the below table. Our method works best when the number of tokens is set to 64. Therefore, we choose 64 as the default number of our approach.\\

\begin{table*}

\centering
\begin{tabular}{cc}
\toprule
Number & Frame-wise acc \\
\hline 
32  & 66.14 \\   
64 & \textbf{67.78}\\
128 & 66.53 \\
\bottomrule
\end{tabular}
\label{table:token}
\end{table*}

\section{Visualization}
\label{sec:vis}
In this section, we provide some visualization results to show the effectiveness of our approach.
\begin{figure}[htbp]
\centering\includegraphics[width=12cm]{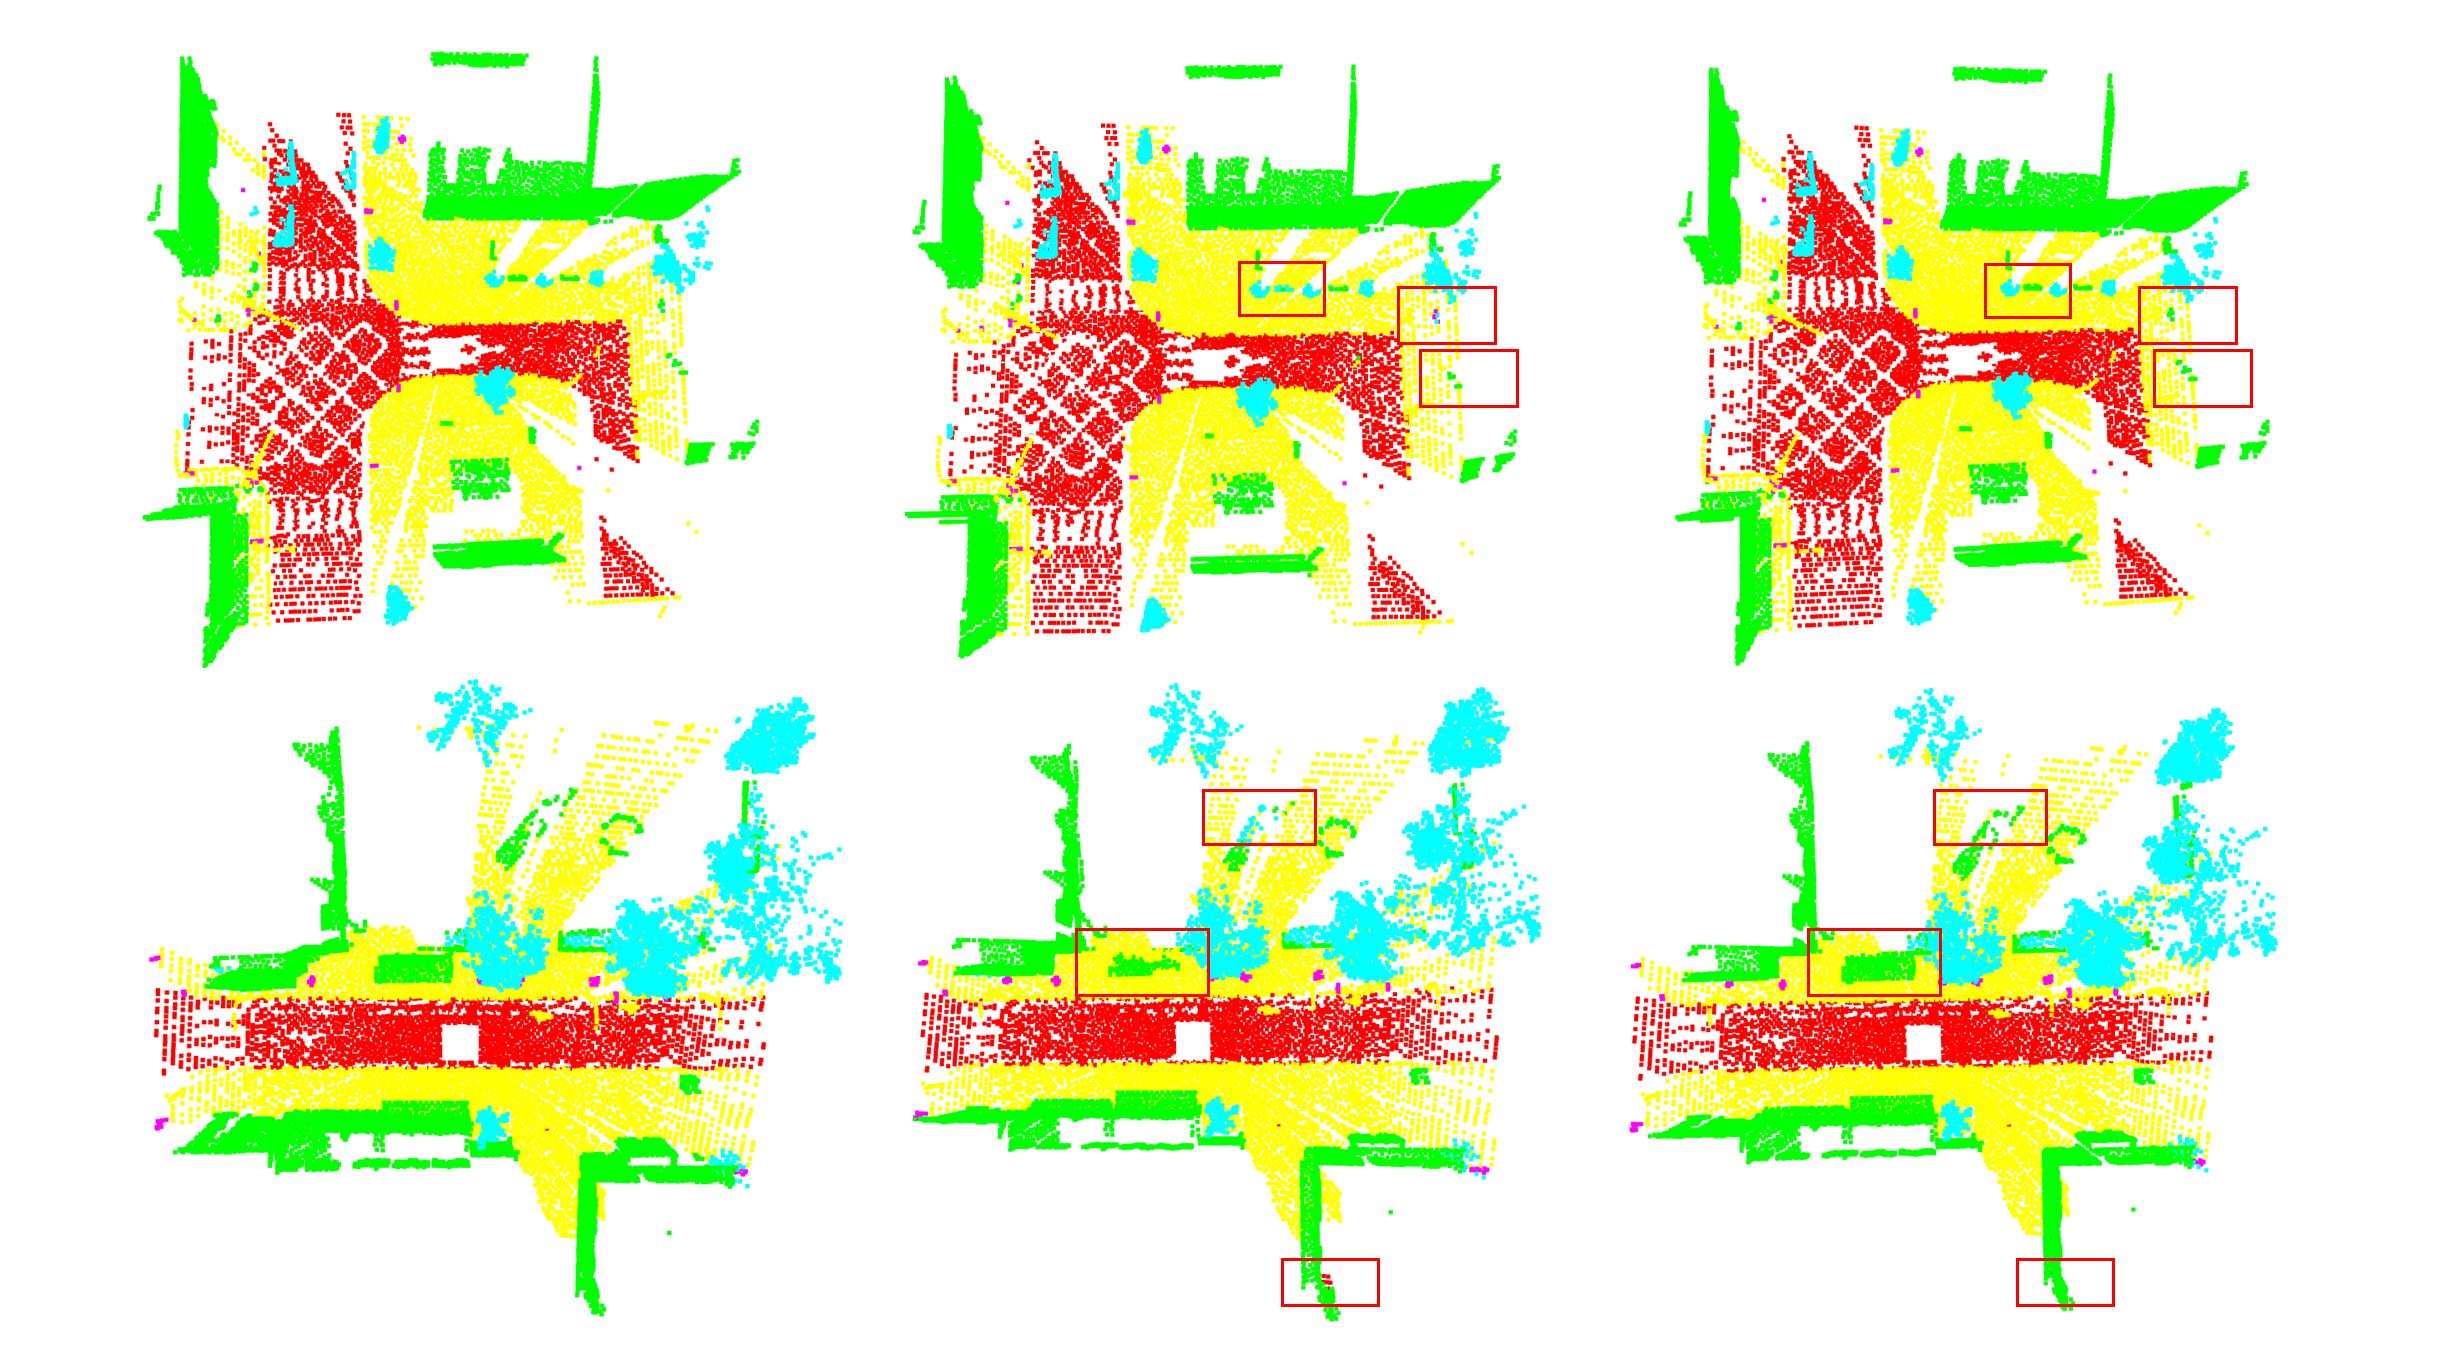}
\caption{Visualization results on Synthia4D dataset.}
\label{figure:vis}
\end{figure}
As shown in Figure~\ref{figure:vis}, we use PPTr as the backbone model. From left to right is the ground truth label, segmentation results of vanilla PPTr and segmentation results of PPTr+NSM4D. The visualization results further shows that the proposed NSM4D is capable of aggregating geometry and motion information from the historical sequences.
% We visualize the anchor points of geometry tokens in the neural scene model. For better visualization, we rotate each frame back to the coordinate of the first frame and use the accumulated points in the first frame's coordinate as the background. As shown in Figure\ref{figure:vis token}, the blue points are the accumulated points, and the red points represent the anchor points. As the number of frames increases, the blue points can gradually reconstruct the complete geometry better. With the deformation flow as good guidance for token-wise geometry update, the anchor points can always cover the whole scene, indicating that the tokens in the neural scene model are not only able to represent geometric information of the current frame but also integrates historical observations through deformation flow to form a complete geometry understanding.
% \begin{figure}[!htbp]
% \centering
% \begin{minipage}[t]{0.3\textwidth}
% \centering
% \includegraphics[width=4.5cm]{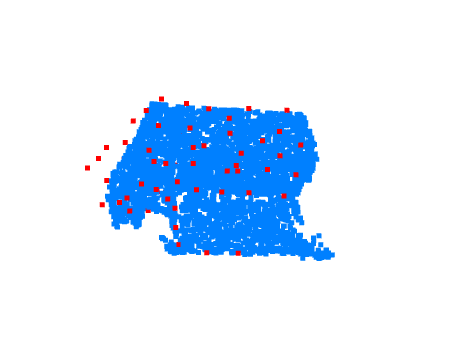}
% \subcaption{25th frame}
% \label{figure:test longer}
% \end{minipage}
% \begin{minipage}[t]{0.3\textwidth}
% \centering
% \includegraphics[width=4.5cm]{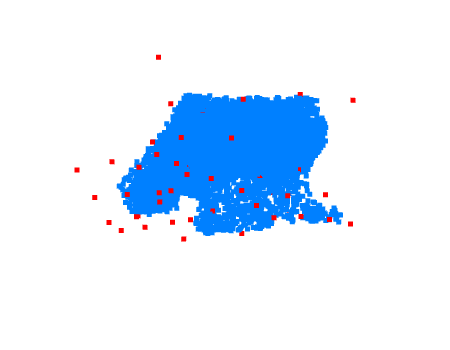}
% \subcaption{80th frame}
% \label{figure:train longer}
% \end{minipage}
% \begin{minipage}[t]{0.3\textwidth}
% \centering
% \includegraphics[width=4.5cm]{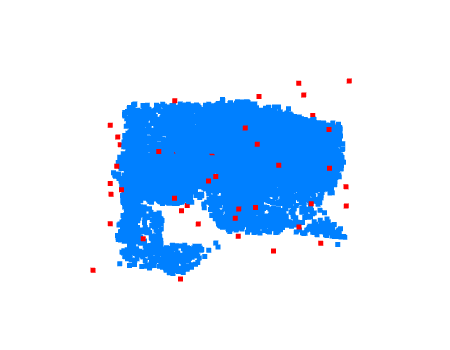}
% \subcaption{149th frame}
% \label{figure:train longer}
% \end{minipage}
% \caption{Visualization of geometry tokens}
% \label{figure:vis token}
% \end{figure}

\section{Implementation Details}
\label{sec:imp}
This section introduces the details of implementing HOI4D action segmentation experiments.

We use SGD to train the neural network. The learning rate is set to be 0.02, and we use a warm-up learning rate scheduler for the first ten epochs, where the learning rate increases linearly. As for parameters, the feature dimension of the neural scene model is chosen to be 1024. For 4D convolution, we use ball query with a radius of 0.9, and the number of samples is set to 32. We adopt learning rate decay at 35, 60, and 80 epochs to achieve better performance by default. With batch size set to 8, our method can be implemented on two NVIDIA A100 40G when training with 150-frame sequences. 

% \section{Broader Impacts}
% \label{sec:broader}
% We propose a new paradigm for online 4D perception based on a neural scene model. Our method has the potential to be applied to robot perception, where the robot needs to understand the time-varying environment for better control and decision-making. Moreover, our method can also help the decision system with the dense perception of the current scene in autonomous driving. However, training our model requires a lot of GPU resources, releasing large amounts of carbon dioxide and contributing to global warming.

\section{Limitations and Future Work}
\label{sec:lim}
Despite the impressive results, our work still has some limitations. First, NSM4D is customized for 4D online perception, but it is still unable to achieve real-time perception due to the computation overhead. We will reduce compute bottleneck and accelerate inference to get real-time dense perception. Also, the proposed neural scene model is purely point-based. If given RGBD sequences as input, how to leverage the fine-grained details in RGB sequences to form a more detailed geometry understanding and more accurate point correspondences in the neural scene model remains to be explored in the future.
